# Supplementary material for: Temperature dependence of the electronic structure and Fermi-surface reconstruction of Eu(1-x)Gd(x)O through the ferromagnetic metal-insulator transition
Source: arXiv:1207.4490 source file (2012-07-18)
Supplement: Supplementary file 1 [file EuO_SupplementaryInformation.pdf]

# Supplementary Information
# Temperature dependence of the electronic structure and Fermi-surface reconstruction of $Eu_{1-x}Gd_xO$ through the ferromagnetic metal-insulator transition

D.E. Shai,[1] A.J. Melville,[2] J.W. Harter,[1] E.J. Monkman,[1]
D.W. Shen,[1] A. Schmehl,[3] D.G. Schlom,[2,4] and K.M. Shen[1,4,*]

[1]*Laboratory of Atomic and Solid State Physics, Department of Physics, Cornell University, Ithaca, New York 14853, USA*
[2]*Department of Materials Science and Engineering, Cornell University, Ithaca, New York 14853, USA*
[3]*Zentrum für elektronische Korrelation und Magnetismus, Universität Augsburg, Universitätsstraße 1, 86159 Augsburg, Germany*
[4]*Kavli Institute at Cornell for Nanoscale Science, Ithaca, New York 14853, USA*

## FILM CHARACTERIZATION

*In situ* reflection high-energy electron diffraction (RHEED) was used to monitor the growth of companion $Eu_{1-x}Gd_xO$ films grown immediately before or after those used in this study. Exemplary RHEED images are shown in Fig. S1(a) for a bare $YAlO_3$ substrate and in Fig. S1(b) for a 35 nm thick film of $Eu_{0.95}Gd_{0.05}O$. The RHEED shows no evidence of second phases or excessive surface roughness.

After the completion of the film growth, the surface crystallinity was further characterized by low-energy electron diffraction (LEED). Exemplary LEED images are shown in Fig S2. The LEED image clearly shows a (001) film surface with no reconstruction.

A companion series $Eu_{1-x}Gd_xO$ films grown under identical conditions to those used in the ARPES study were used to perform *ex situ* x-ray diffraction and x-ray absorption spectroscopy (XAS). XAS measurements were used to precisely determine the Gd content and oxidation states and were performed at the SGM beamline at the Canadian Light Source, following the method of Sutarto *et al.* [S1]. Films with nominal Gd content $x = 0$, 0.02, 0.08, and 0.16 were grown and were then capped with 20 nm amorphous Silicon to prevent oxidation of the film. Uncapped EuO

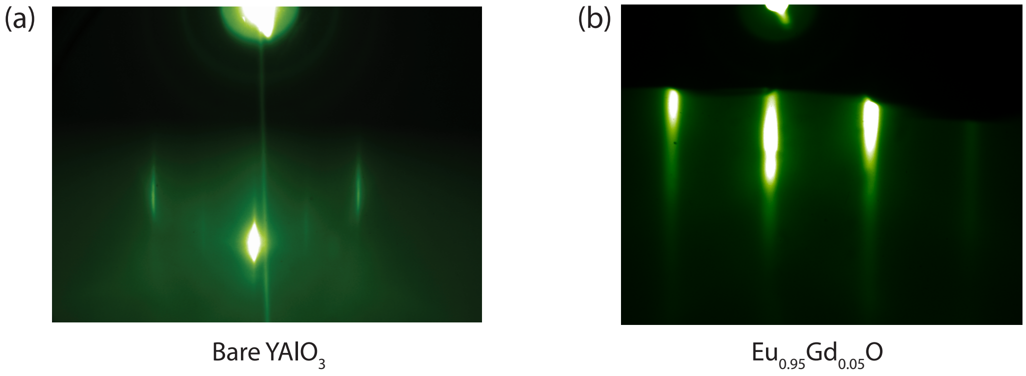


Figure S1: Reflection high-energy electron diffraction (RHEED) pattern for (a) bare $YAlO_3$ substrate and (b) 35nm $Eu_{0.95}Gd_{0.05}O$ film.

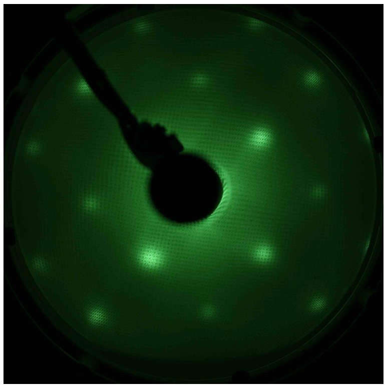

Figure S2: Low-energy electron diffraction (LEED) image of an $Eu_{0.95}Gd_{0.05}O$ film grown on $YAlO_3$. The electron beam energy is 100 eV.

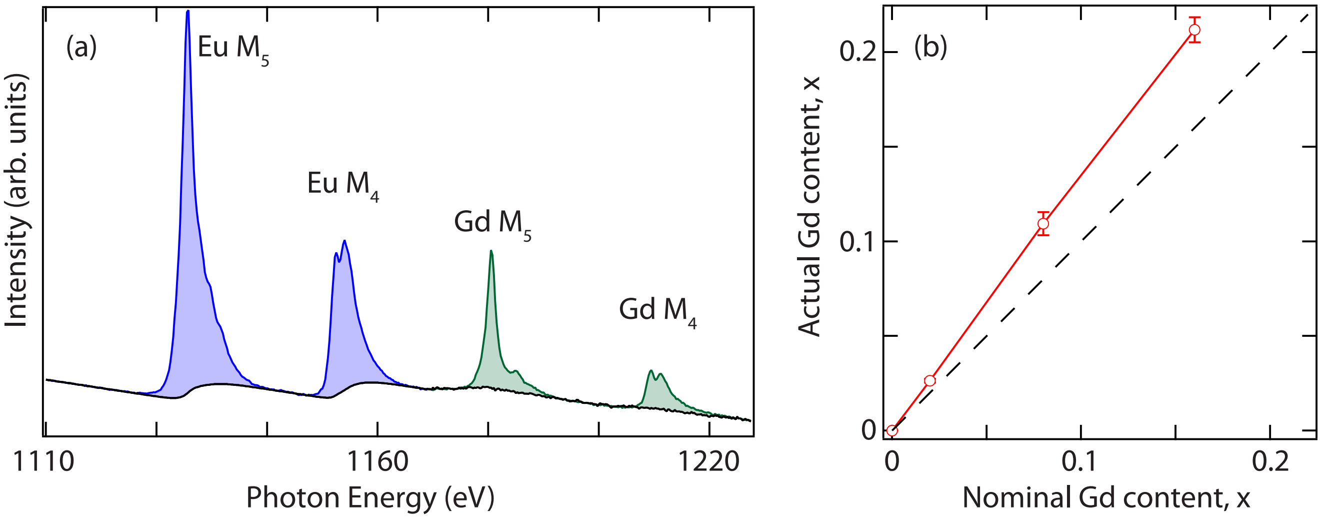


Figure S3: (a) Example XAS spectrum for an $x = 0.21$ film. (b) Calibration of actual Gd content determined by XAS against nominal film Gd content.

films degrade in air nearly instantaneously. XAS was performed on the Eu and Gd $M_{4,5}$ edges. For each film, the total electron yield was recorded as the photon energy was varied between 1100 and 1245 eV. An empirical Shirley background and the extended x-ray absorption fine structure (EXAFS) were then removed from the spectra. Fig. S3 (a) shows an example absorption spectrum for a nominal doping of $x = 0.16$. The spectra are consistent with all Gd being in the 3+ oxidation state, despite our measurements indicating a large number of inactive dopants. To determine the actual Gd content, the area beneath the Gd $M_{4,5}$ edges (green area in Fig. S3a) was divided by the integrated area beneath both the Eu and Gd edges (green and blue areas in Fig. S3a). The actual Gd content for each of these samples was calculated and is shown in Fig. S3 (b).

The companion series were further characterized by x-ray diffraction. $\theta - 2\theta$ scans are shown in Fig. S4 for samples with a measured Gd content of $x = 0.007$, 0.013, and 0.05. All films are (001) oriented and show no evidence of extra

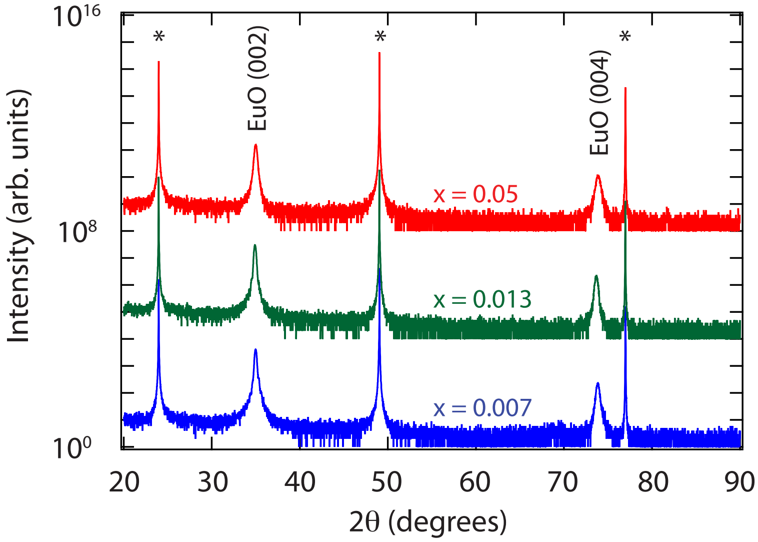


Figure S4: X-ray diffraction $\theta - 2\theta$ scans for $x = 0.007$, 0.013, and 0.05 showing phase pure, oriented (001) films.

phases.

## ELECTRONIC STRUCTURE CALCULATIONS

Density functional theory calculations of the band structure and Fermi surface of $Eu_{1-x}Gd_xO$ were performed using the WIEN2k software package [S2]. An on-site Coulomb repulsion and exchange parameter was applied to the Eu 4f orbitals ($U_f = 8.3$ eV, $J_H = 0.77$ eV) and the O 2p orbitals ($U_p = 4.6$ eV, $J_H = 1.2$ eV), after Ref. S3. The relaxed lattice constant of the cubic fcc unit cell was found to be $a = 5.166$ Å. The Fermi level was shifted into the conduction band by 475 meV, corresponding to a doping of $x = 0.025$ (50% active carriers in a film with nominal $x = 0.05$ doping).

The simulated ARPES Fermi surface was generated by averaging the calculated Fermi surface along $k_z$, weighted with a Lorentzian of width $1/\lambda$, where $\lambda = 8$ Å is the photoelectron mean free path. The location in $k_z$ was determined based on the synchrotron-based photoemission measurements in Ref. S4, wherein it was reported that at $(k_x, k_y) = (0, 0)$, states near $k_z = 6\pi/c$ (the $X$ point in the extended fcc Brillouin zone) are probed with 38 eV photons, and states at $k_z = 8\pi/c$ (the $\Gamma$ point in the extended fcc Brillouin zone) are probed with 78 eV photons.

In the context of the nearly free electron model [S5], the location probed in $k_z$ is given by

$$k_z = \sqrt{\frac{2m}{\hbar^2}(E_{h\nu} + V_0 - \phi) - k_{\parallel}^2}, \tag{S1}$$

where $E_{h\nu}$ is the photon energy, $\phi$ is the work function, and $k_{\parallel}$ is the in-plane component of the electron momentum.

Combining eq. (S1) and the photoemission measurements discussed above, the inner potential for EuO is $V_0 - \phi = 13.2$ eV.

## COMPARISON BETWEEN CALCULATIONS AND PHOTOEMISSION DATA WITH PHOTON ENERGY = 40.8 EV

To confirm the accuracy of the inner potential discussed above, we have additionally measured the electronic structure of EuO probed with 40.8 eV light (He II), which probes near $k_z = 2\pi/c$. As is illustrated in Fig. S5, the calculated ARPES Fermi surface at this photon energy appears qualitatively different than that calculated for 21.2 eV light (Fig 3(c) in the main text). The electron pocket occurring at $X$ is observable as a ring of intensity about $k_x = k_y = 0$. Additionally, while elliptical electron pockets still exist at $k_x = 2\pi/a$, the orientation of these pockets is rotated by 90 degrees relative to the 21.2 eV calculation. These features originate from electron pockets occurring in the second Brillouin Zone. We have made ARPES measurements along high symmetry lines using 40.8 eV light to compare with these calculations, and the results are shown in Fig. S5.

These measurements exhibit remarkable agreement with the calculated Fermi surface, confirming that our determination of $k_z$ using the inner potential described above is valid. In particular we note that our measurements confirm the existence of an electron pocked at $k_x$ and $k_y = 2\pi/a$, and that this pocket is elongated along the direction of the zone boundary.

It must be noted that the measurements shown in Fig. S5 were taken on films doped with La rather than Gd. While La differs from Gd in valence electron structure, it still behaves qualitatively the same when doped into EuO (e.g., it has a 3+ valence and produces similar transport properties). Additionally, we have confirmed that the data presented in the main text is reproducible using La as a dopant.

## TEMPERATURE DEPENDENT SPECTRA AT THE BRILLOUIN ZONE BOUNDARY

In addition to the near $E_F$ spectra taken at the Brillouin zone boundary (BZB) at 140 K and 10 K presented in the main text, a third set of data was acquired at T = 50 K. Shown in Fig. S6 are energy distribution curves taken at the Brillouin zone boundary at T = 140, 50, and 10 K, and shifted in energy according to the temperature-dependent redshift (see Figs. 1c, d in the main text). The spectra in Fig. S6 illustrate that as the sample is warmed above the Curie temperature, the absence of long-range magnetic order causes the Eu 5d conduction band to lift above the Fermi level, thereby releasing the active carriers into pseudogapped states, as discussed in the main text.

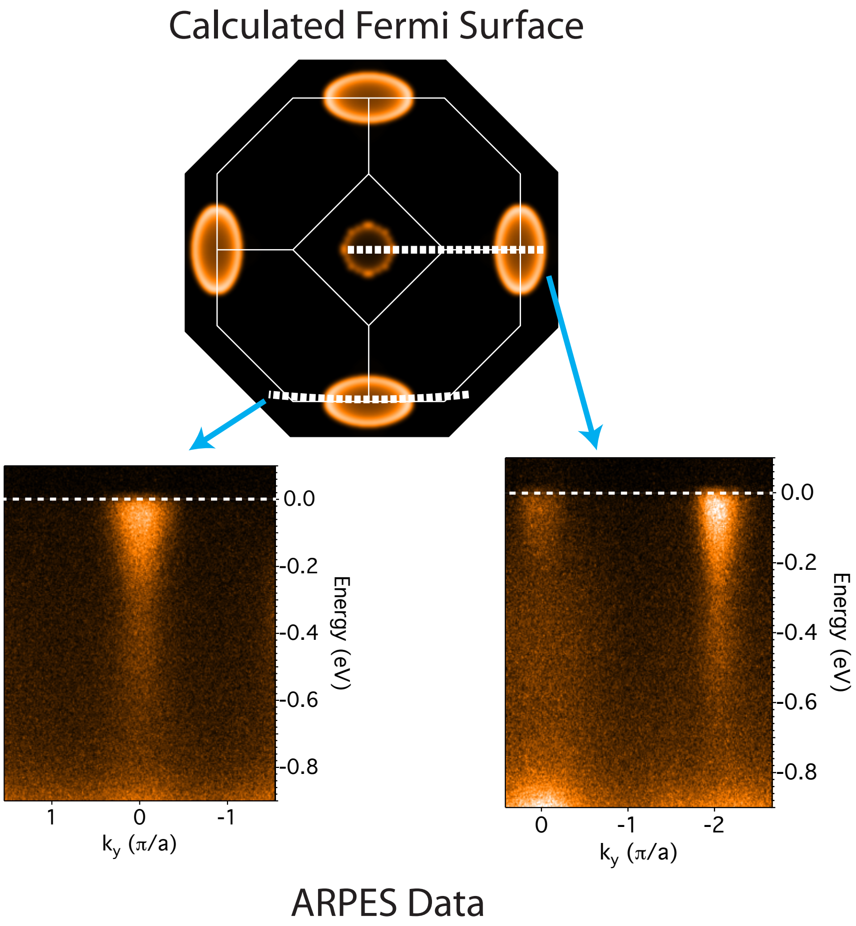


Figure S5: (top) Calculated ARPES Fermi surface for electron-doped EuO using a photon energy of 40.8 eV, which probes near $k_z = 2\pi/c$. (bottom) ARPES data taken on nominally 4% La-doped EuO taken at T = 10 K.

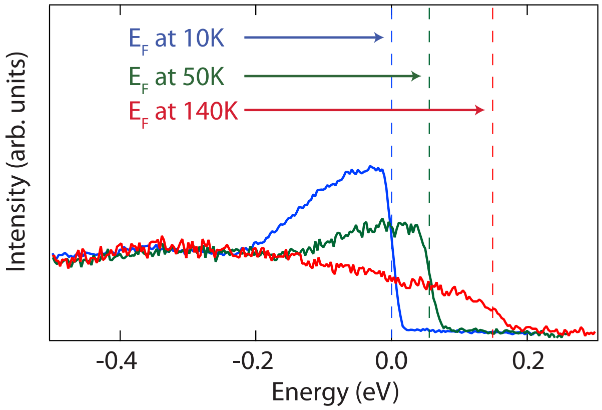


Figure S6: Near-$E_F$ spectra for $Eu_{0.95}Gd_{0.05}O$ integrated within $k_x = \pm 0.25 Å^{-1}$ at the Brillouin zone boundary ($k_y = 2\pi/a$). The spectra taken at $T = 50$ and 140 K are shifted in energy to account for the temperature-dependent redshift, discussed in the main text.

## COMPARISON BETWEEN THE PGS AND DBS

In this section we expand upon our identification of two types of dopant-induced states observed at the Brillouin Zone (BZ) center. At 10K, we observe broad and only weakly dispersive spectral weight in the region around (0, 0), shown in Fig. 2(b)(i) of the main text and reproduced in Fig S7(a) below. The spectral weight decreases to nearly zero at the Fermi level, indicating that these states do not contribute to metallic conduction observed at low temperatures. In contrast, above $T_c$ at 140K we observe an additional component to the spectral intensity around (0, 0) (particularly clear at $k_F$), one which clearly shows dispersion and has small but finite weight at $E_F$. This data, originally shown in Fig 2(d)(iii) in the main text is reproduced in Fig. S7(b). The data in Fig. S7 (a) & (b) have been normalized to the Eu 4f band intensity at 2.25 eV and are plotted on the same color scale.

To better illustrate the differences in spectral lineshapes between the two features, in Fig. 4(b) of the main text and reproduced in Fig. S7(c) & (d) we compare energy distribution curves (EDCs) below and above $T_c$ taken at $k = 0$ and $k = k_F$, where $k_F$ is determined by the peaks in the momentum distribution curve at $E_F$ at 140K (see Fig. 4(a) of the main text). The EDCs in Fig. S7(c) & (d) have been normalized to their peak maximum between 0.2 to 0.5 eV binding energy for better comparison of the lineshape. At low temperatures (S7(c)) the EDCs are nearly identical, highlighting the minimal dispersion and concentration of spectral weight far from $E_F$ (hence our designation of these as deeply bound states (DBS)).

The corresponding EDCs above $T_c$ in Fig. S7(d), are clearly different at $k = 0$ and $k = k_F$, indicating the presence of a strongly dispersive component of spectral weight. This additional component sits closer to $E_F$ than the DBS, but has suppressed intensity within 200 meV of $E_F$. The small but nonzero component of spectral weight at $E_F$ leads us to designate this additional high-temperature component of spectral weight as pseudogapped states (PGS).

To further illustrate the differences between the high and low temperature data at the BZ center, in Fig. S7(e) & (f) we plot EDCs over a wide range of $k$ (as indicated in Fig. S7(a) & (b)). The EDCs have been normalized to their peak intensity, and the $k = 0$ EDC has been subtracted from each. The T = 140 K data in S7(e) clearly shows the contribution from the dispersive PGS, whereas in the T = 10 K S7(f) only a weakly dispersive signal is observed.

While the change in lineshape at $k_F$ illustrated in Fig. S7(c) & (d) prominently shows the additional PGS, the spectrum precisely at $k = (0,\ 0)$ exhibits only minor changes, primarily a shift of 55 meV toward $E_F$. To clarify the PGS contribution to the $k = (0,\ 0)$ EDC lineshape, we have performed measurements on a sample with a slightly higher doping ($x = 0.06$). In Fig. S8, we again show EDCs for the $x = 0.05$ sample along with a $x = 0.06$ (note that in Fig. S8 EDCs are grouped to the same $k$ values, and are not to be confused with Fig 4(b) of the main text, which groups EDCs of identical temperatures). At $x = 0.06$ doping, the PGS contribution to the lineshape at both $k = 0$ and $k = k_F$ is apparent as a shoulder at approximately 150 meV, indicating that the PGS forms a continuous band with spectral intensity at $k = 0$.

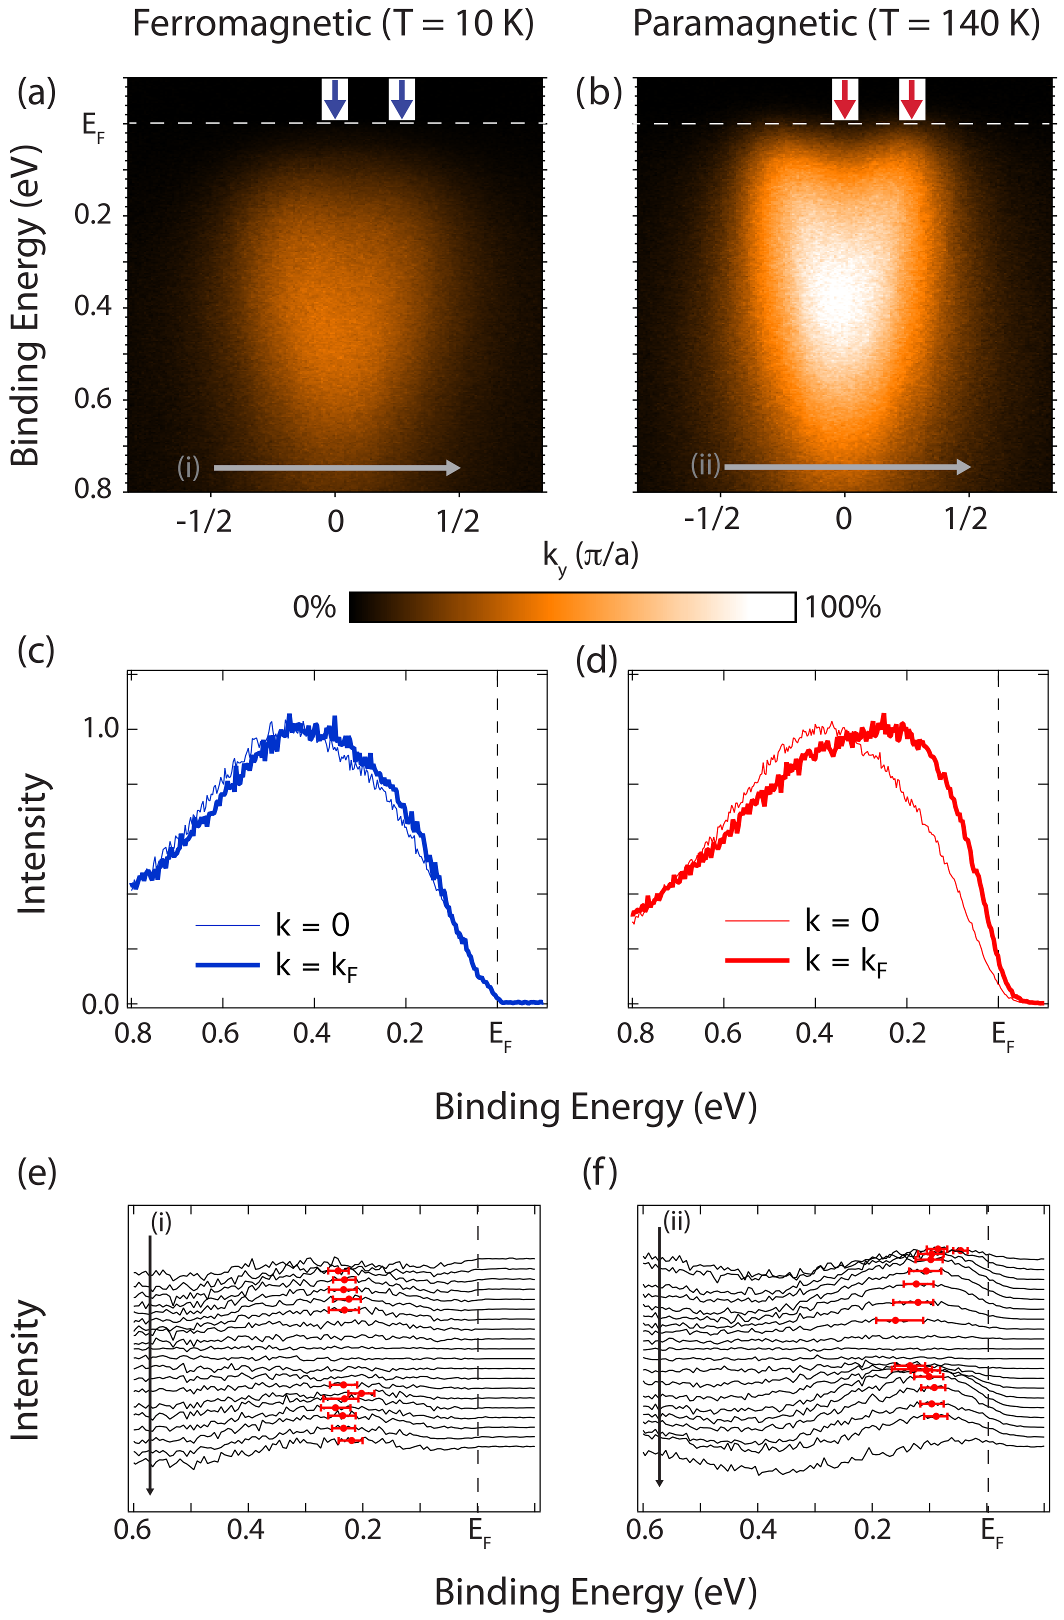


Figure S7: E versus k spectra for $Eu_{0.95}Gd_{0.05}O$ taken at the Brillouin Zone center (a) below and (b) above $T_c$, showing the distinction between PGS (above $T_c$) in addition to the DBS (present at all temperatures). The intensity has been normalized to the Eu 4f band. (c) T = 10 K EDCs at $k = 0$ and $k = k_F$ normalized to their peak maxima, showing minimal dispersion and lack of near-$E_F$ spectral weight of the DBS. (d) T = 140 K EDCs at $k = 0$ and $k = k_F$ normalized to their peak maxima showing dispersive spectral weight of the PGS approaching $E_F$. (e) & (f) EDCs normalized to their peak maxima, with the $k = 0$ spectrum subtracted. Red markers indicate peaks in the EDCs where discernible.

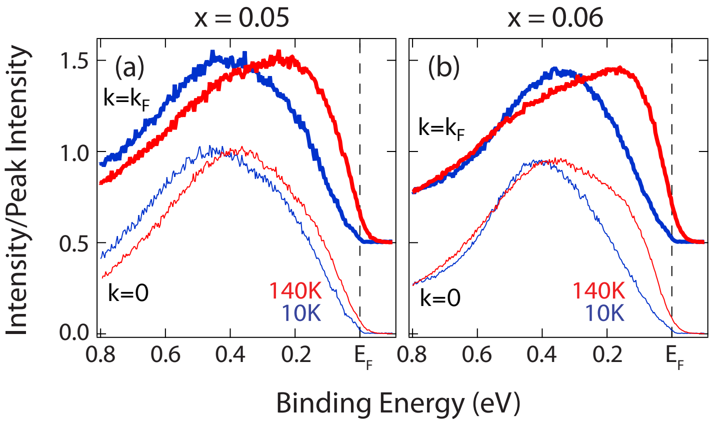


Figure S8: Temperature-dependent EDCs taken at the BZ center on $Eu_{1-x}Gd_xO$ with Gd doping levels $x$ of (a) 0.05 and (b) 0.06. EDCs have been normalized to their peak intensity between 0.2-0.5 eV binding energy to illustrate differences in lineshape.

## CALCULATION OF THE NUMBER OF ACTIVE CARRIERS

The percentage of dopants that enter pseudogapped states (PGS) and in gap states (IGS) can be estimated by comparing the photoemission intensity about the BZ center at T = 10 K and 140 K (Fig. 2c and 2f in the main text). The data was integrated in energy over the near-$E_F$ states to produce momentum distribution curves of the dopant-induced states below $E_F$. These curves represent the photoemission intensity along a 1-dimensional line through the 3-dimensional Brillouin zone. Assuming a spherical geometry and that $k_z = 0$, the total photoemission intensity $I$ at a given temperature $T$ can be represented as an integral of the momentum distribution curve at that temperature, $MDC_T(k)$:

$$\begin{aligned} I(T) &= \iiint MDC_T(k)\ k^2 \sin(\theta) dk d\theta d\phi \\ &\approx 2\pi \int_{-\pi/a}^{\pi/a} MDC_T(k)\ k^2 dk. \end{aligned} \tag{S2}$$

By comparing the spherically-integrated number of states at 140 K and 10 K, the number of dopants entering MPS be computed as

$$\text{Active dopants} = \frac{I(140) - I(10)}{I(140)}. \tag{S3}$$

Using the data shown in Fig. 2c and 2f in the main text, we find that 50 ± 10% of the dopants enter PGS, while the remaining carriers enter the inactive IGS.

* Author to whom correspondence should be addressed: kmshen@cornell.edu

[S1] R. Sutarto *et al.*, Phys. Rev. B **80,** 085308 (2009)

[S2] P. Blaha *et al.*, *WIEN2k: An Augmented Plane Wave Plus Local Orbitals Program for Calculating Crystal Properties* (TU Wien, Austria, 2001).

[S3] N.J.C. Ingle and I.S. Elfimov, Phys. Rev. B **77,** 121202(R) (2008).

[S4] H. Miyazaki *et al.*, Phys. Rev. Lett. **102,** 227203 (2009).

[S5] A. Damascelli, Phys. Scripta **T109,** 61 (2004).
